# Supplementary material for: On the Theory of Policy Gradient Methods: Optimality, Approximation, and Distribution Shift
Source: arXiv:1908.00261 source file (2020-10-14)
Supplement: Supplementary file 1 [file appendix_compatible.tex]

\section{Compatible Function Approximation and Policy Gradients}
\label{app:compatible}

It may help the reader to recall the compatible fucntion approximation result of~\cite{sutton1999policy}. Consider the state-action
visitation distribution under $\pi$ starting from $\mu$, i.e.
\[
  \nu(s,a)=  d_{\mu}^{\pi_\theta}(s) \pi_\theta(a | s)
  \]
and the minimizer
\begin{equation*}
w^\star(\theta) \in \argmin_w L_\nu(w;\theta).
\end{equation*}
Let us denote the best linear predictor of $A^{\pi_\theta}(s,a)$ using
$\nabla_\theta \log \pi_\theta(a | s)$ by $\widehat
A^{\pi_\theta}(s,a)$, i.e. 
\[
\widehat A^{\pi_\theta}(s,a) := w^\star(\theta) \cdot \nabla_\theta \log \pi_\theta(a | s).
\]
As shown in ~\cite{sutton1999policy}, the first order optimality conditions for
$\widehat A^{\pi_\theta}(s,a)$ being the best linear predictor
directly imply that:
\begin{eqnarray*}
  \nabla_\theta V^{\pi_\theta}(\mu) &=&
\frac{1}{1-\gamma} \, \E_{s \sim d_{\mu}^{\pi_\theta} }\E_{a\sim \pi_\theta(\cdot | s) }
\big[\nabla_\theta \log \pi_{\theta}(a| s) A^{\pi_\theta}(s,a)\big]\\
&=&
\frac{1}{1-\gamma} \, \E_{s \sim d_{\mu}^{\pi_\theta} }\E_{a\sim \pi_\theta(\cdot | s) }
\big[\nabla_\theta \log \pi_{\theta}(a| s) \widehat A^{\pi_\theta}(s,a)\big].
\end{eqnarray*}
In other words, computing the gradient with the best linear
approximation, $\widehat A^{\pi_\theta}(s,a)$, instead of
$A^{\pi_\theta}(s,a)$ results in identical outcomes.
